# Supplementary material for: Inversion in a four-terminal superconducting device on the quartet line: I. Two-dimensional metal and the quartet beam splitter
Source: arXiv:2008.01981 ancillary file (2020-12-13)
Supplement: Supplementary file 1 [file revised_supplemental_material_final3.pdf]

# Inversion in a four terminal superconducting device on the quartet line: I. Two-dimensional metal and the quartet beam splitter Supplemental Material

Régis Mélin[1]

[1] *Univ. Grenoble-Alpes, CNRS, Grenoble INP, Institut NEEL, 38000 Grenoble, France*

The Supplemental Material contains technical details of the calculations.

The Supplemental Material is organized as the following. Section I presents a sanity check of Eqs. (16)-(19) in the paper. Section II of the Supplemental Material details the calculations of the critical currents from perturbation theory in the tunnel amplitudes (see section V in the paper). A relation used in section VIII B of the paper is demonstrated in section III of the Supplemental Material.

## I. SANITY CHECK OF EQS. (16)-(19) IN THE PAPER

In this section, Eqs. (16)-(19) in the paper are illustrated on the simple example of a 2D metal forming two contacts with normal leads. This calculation shows that Eqs. (16)-(19) in the paper have physically acceptable consequences.

Figure 1 shows schematically single-channel contacts between a 2D metal and two normal tips supposed to form tunnel junctions. Both tips and the 2D metal are described by a tight-binding model. The corresponding tight-binding sites are denoted by $(a,\alpha)$ and $(b,\beta)$, where $a$, $b$ are the contact points on both tip and $\alpha$, $\beta$ are their counterparts on the 2D metal. The Dyson Eq. (23) in the paper yields

$$G^A_{a,a} \simeq g^A_{a,a}\left[1+J_{a,\alpha}g^A_{\alpha,\beta}J_{\beta,b}g^A_{b,b}J_{b,\beta}g^A_{\beta,\alpha}J_{\alpha,a}g^A_{a,a}\right], \quad (1)$$

where $G_{a,a}$ is the Green's function at the tight-binding site $a$, dressed at lowest order by the coupling to $N_b$ through the 2D metal, and $g_{i,j}$ denotes the Green's functions with all tunnel amplitudes $J_{a,\alpha}=J_{\alpha,a}=J_{b,\beta}=J_{\beta,b}=0$ set equal to zero.

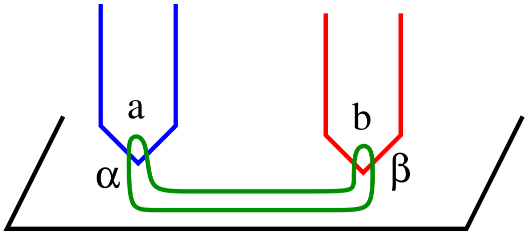


FIG. 1. Schematics of the two-terminal configuration used as a toy-model to illustrate the emergence of advanced-advanced or retarded-retarded transmission modes through the 2D metal, and to verify that their sign is correct, see Eqs. (16)-(19) in the paper.

Using $g^A_{a,a}=i/W_a$, $g^A_{b,b}=i/W_b$ (where $W_a$ and $W_b$ denote the band-width in the normal tips $N_a$ and $N_b$) yields

$$G^A_{a,a} \simeq \frac{i}{W_a}\left[1-\frac{|J_{\alpha,a}|^2|J_{\beta,b}|^2 g^A_{\alpha,\beta}g^A_{\beta,\alpha}}{W_aW_b}\right], \quad (2)$$

where $g^A_{\alpha,\beta}g^A_{\beta,\alpha}$ denotes an advanced-advanced mode between the tight-binding sites $\alpha$ and $\beta$.

Eqs. (16)-(17) in the paper imply that the product $g^A_{\alpha,\beta}(R)g^A_{\beta,\alpha}(R)$ is real-valued and negative, whatever the separation $R$ between the contacts.

The above Eq. (2) is interpreted as the following: $N_b$ reduces the energy level spacing on $N_a$ by introducing a coupling to its density of energy levels. Thus, the density of states at $N_a$ is enhanced by the coupling to $N_b$ and the "$i$" coefficient in Eq. (17) in the paper implies the expected positive coupling between the density of states of both tips. We conclude that Eqs. (16)-(19) in the paper have passed a sanity test.

Now, we continue the discussion and assume that the $(a,\alpha)$ and the $(b,\beta)$ single channel contacts are replaced by more extended interfaces. Eq. (2) becomes

$$G^A_{a_p,a_p} \simeq \frac{i}{W_a}\left[1-\sum_q\frac{|J_{\alpha_p,a_p}|^2|J_{\beta_q,b_q}|^2 g^A_{\alpha_p,\beta_q}g^A_{\beta_q,\alpha_p}}{W_aW_b}\right], \quad (3)$$

where $p$ and $q$ label the tight-bing sites at the interfaces in real space. For simplicity, we ignore nonlocality in $N_a$ and $N_b$. Namely, a spin-up electron entering $N_a$ or $N_b$ at the tight-binding site $p$ necessarily exits at the same $p$ instead of a different $p'\neq p$. The following argument can however be generalized to $N_a$ and $N_b$ not consisting of a collection of independent 1D channels.

Assuming now that $|J_{\alpha_p,a_p}|\equiv|J_{\alpha,a}|$ and $|J_{\beta_q,b_q}|\equiv|J_{\beta,b}|$ are independent on $p$ and $q$ respectively yields

$$G^A_{a_p,a_p} \simeq \frac{i}{W_a}\left[1-\frac{|J_{\alpha,a}|^2|J_{\beta,b}|^2\sum_q\left(g^A_{\alpha_p,\beta_q}g^A_{\beta_q,\alpha_p}\right)}{W_aW_b}\right]. \quad (4)$$

Then, $\sum_q\left(g^A_{\alpha_p,\beta_q}g^A_{\beta_q,\alpha_p}\right)$ can be approximated as the following:

$$\sum_q\left(g^A_{\alpha_p,\beta_q}g^A_{\beta_q,\alpha_p}\right) \quad (5)$$

$$\simeq N_{ch}\frac{k_F}{2\pi}\int_{R_0}^{R_0+2\pi/k_F}\left[g^A(R)\right]^2 dR \quad (6)$$

$$\simeq -\frac{N_{ch}}{2\pi W^2R_0}\int_{R_0}^{R_0+2\pi/k_F}\left[\cos\left(k_FR-\frac{\pi}{4}\right)\right]^2 dR \quad (7)$$

$$\simeq -\frac{N_{ch}}{2k_FR_0W^2}, \quad (8)$$

where we used Eqs.(16)-(17) in the paper, and $N_{ch}$ denotes the number of "channels" at the 2D metal-$N_b$ interface. Thus,

a 2D metal couples coherently two normal leads $N_a$ and $N_b$ attached to it, within range limited by the phase-coherence length $l_\varphi$.

The above Eqs (4)-(8) are in correspondance with Eq. (94) in the paper.

We note in passing the consequences for the ferromagnetic proximity effect in ferromagnet-graphene-ferromagnet spin valves. Magnetization is predicted to penetrate the 2D metal over long distance $l_\varphi$. However, providing experimental evidence seems to be challenging.

## II. EVALUATION OF THE ORDER-$(J_0/W)^{12}$ CONTRIBUTIONS TO THE ADIABATIC-LIMIT 4TSQ CURRENT

### A. Evaluation of the subleading order-$\sqrt{\mathscr{S}_{contact}}/l_e$ contribution

The following expressions provide an expansion of $\left(\hat{J}_{a,\alpha}\hat{G}_{\alpha,a}\right)$, which is one of the terms contributing to the 4TSQ current in the adiabatic limit, see Eqs. (34)-(37) in the paper.

All diagrams are enumerated at the order $(J_0/W)^{12}$. A selection of the diagrams appearing in perturbation is operated, keeping only the following two contributions:

(i) The diagrams contributing to the dc-component of $\left(\hat{J}_{a,\alpha}\hat{G}_{\alpha,a}\right)$.

(ii) The diagrams which allow for gathering the Green's functions through the 2D metal in a pair-wise manner.

The notations for $\left(\hat{J}_{a,\alpha}\hat{G}_{\alpha,a}\right)$ are the same as in the paper:

(i) We use $(n_a, n_b, n_{c,1}, n_{c,2})$ in the superscript for the sensitivity on the superconducting phase variables, according to Eq. (48) in the text of the paper.

(ii) In the subscript, the notations [8] or [12] refer to the orders $(J_0/W)^8$ or $(J_0/W)^{12}$ at which $\left(\hat{J}_{a,\alpha}\hat{G}_{\alpha,a}\right)$ is evaluated in perturbation.

Specifically, the formula presented here in the Supplemental Material detail the expression of the critical current at the order $(J_0/W)^{12}$. The order $(J_0/W)^8$ is presented in sections IV A and IV B of the paper.

(iii) The labels $(1,1)$ and $(2,2)$ in the subscript refer to spin-up electron and spin-down holes respectively.

(iv) The (1) or (2) labels refer to the contributions to the critical current which are proportional to $\sqrt{\mathscr{S}_{contact}}/l_e$ or to $\mathscr{S}_{contact}/l_e^2$ respectively, where $\mathscr{S}_{contact} = \pi r_0^2$ is the area of the contacts between the 2D metal and the superconducting leads, see the device geometry and the notation $r_0$ on figure 3c in the paper.

Concerning the above item (iv), we assume that each of the contact with the superconducting leads $S_a$, $S_b$, $S_{c,1}$ and $S_{c,2}$ has a different radius $R_a$, $R_b$, $R_{c,1}$ and $R_{c,2}$ which is smaller than the zero-energy dirty-limit superconducting coherence length $\xi_{dirty}(0)$ given by Eq. (53) in the paper, see also section IV C in the paper for the discussion of $r_0 \lesssim \xi_{dirty}(0)$ or $r_0 \gtrsim \xi_{dirty}(0)$, where the notation $r_0$ stands for $R_a$, $R_b$, $R_{c,1}$ and $R_{c,2}$ taken as being identical, *i.e.* $r_0 = R_a = R_b = R_{c,1} = R_{c,2}$.

The product of three Green's functions appearing in the contributions of order $\sqrt{\mathscr{S}_{contact}}/l_e$ is evaluated from the Wick theorem according to Appendix D 4 in the paper.

#### 1. *Spin-up electron/spin-up electron* $(1,1)$ *Nambu component*

Now, we detail the terms contributing to Eq. (74) in the paper:

$$\langle\langle J_{(a,\alpha),(1,1)} G^{A,(-1,-1,1,1)}_{[12],(\alpha,a),(1,1),(1)} \rangle\rangle = \sum_{\lambda=1}^{10} \langle\langle J_{(a,\alpha),(1,1)} G^{A,(-1,-1,1,1)}_{[12],(\alpha,a),(1,1),(1),\lambda} \rangle\rangle, \tag{9}$$

where the $\lambda = 1, ..., 10$ terms $\langle\langle J_{(a,\alpha),(1,1)} G^{A,(-1,-1,1,1)}_{[12],(\alpha,a),(1,1),(1),\lambda} \rangle\rangle$ contribute to the "$(1,1)$" Nambu component, and they are listed according to

$$\langle\langle J_{(a,\alpha),(1,1)} G^{A,(-1,-1,1,1)}_{[12],(\alpha,a),(1,1),(1),1} \rangle\rangle = J_0^{12} \langle\langle g^{A,1,1}_{\alpha,\gamma_{c_1}} g^{A,1,2}_{c_1,c_1} g^{A,2,2}_{\gamma_{c_1},\alpha} g^{A,2,1}_{a,a} g^{A,1,1}_{\alpha,\gamma_{c_2}} g^{A,1,2}_{c_2,c_2} g^{A,2,2}_{\gamma_{c_2},\alpha} g^{A,2,2}_{a,a} g^{A,2,2}_{\alpha,\beta} g^{A,2,1}_{b,b} g^{A,1,1}_{\beta,\alpha} g^{A,1,1}_{a,a} \rangle\rangle \tag{10}$$

$$= J_0^{12} \langle\langle g^{A,1,1}_{a,a} g^{A,2,1}_{a,a} g^{A,2,2}_{a,a} \rangle\rangle \langle\langle g^{A,2,1}_{b,b} \rangle\rangle \langle\langle g^{A,1,2}_{c_1,c_1} \rangle\rangle \langle\langle g^{A,1,2}_{c_2,c_2} \rangle\rangle \langle\langle g^{A,2,2}_{\alpha,\beta} g^{A,1,1}_{\beta,\alpha} \rangle\rangle \langle\langle g^{A,1,1}_{\alpha,\gamma_{c_1}} g^{A,2,2}_{\gamma_{c_1},\alpha} \rangle\rangle \langle\langle g^{A,1,1}_{\alpha,\gamma_{c_2}} g^{A,2,2}_{\gamma_{c_2},\alpha} \rangle\rangle \tag{11}$$

$$= \frac{c_{1/2}}{16} \left(\frac{J_0}{W}\right)^{12} \frac{R_a}{l_e} \frac{1}{k_F R_{\alpha,\beta}} \frac{1}{k_F R_{\alpha,\gamma_{c,1}}} \frac{1}{k_F R_{\alpha,\gamma_{c,2}}} \frac{\Delta^6}{\left(\Delta^2 - (\omega - i\eta)^2\right)^3} \exp\left[i\left(-\varphi_a - \varphi_b + \varphi_{c_1} + \varphi_{c_2}\right)\right] \tag{12}$$

$$\langle\langle J_{(a,\alpha),(1,1)} G^{A,(-1,-1,1,1)}_{[12],(\alpha,a),(1,1),(1),2} \rangle\rangle = J_0^{12} \langle\langle g^{A,1,1}_{\alpha,\gamma_{c_1}} g^{A,1,2}_{c_1,c_1} g^{A,2,2}_{\gamma_{c_1},\alpha} g^{A,2,2}_{a,a} g^{A,2,2}_{\alpha,\beta} g^{A,2,1}_{b,b} g^{A,1,1}_{\beta,\alpha} g^{A,1,1}_{a,a} g^{A,1,1}_{\alpha,\gamma_{c_2}} g^{A,1,2}_{c_2,c_2} g^{A,2,2}_{\gamma_{c_2},\alpha} g^{A,2,1}_{a,a} \rangle\rangle \tag{13}$$

$$= J_0^{12} \langle\langle g^{A,1,1}_{a,a} g^{A,2,1}_{a,a} g^{A,2,2}_{a,a} \rangle\rangle \langle\langle g^{A,2,1}_{b,b} \rangle\rangle \langle\langle g^{A,1,2}_{c_1,c_1} \rangle\rangle \langle\langle g^{A,1,2}_{c_2,c_2} \rangle\rangle \langle\langle g^{A,2,2}_{\alpha,\beta} g^{A,1,1}_{\beta,\alpha} \rangle\rangle \langle\langle g^{A,1,1}_{\alpha,\gamma_{c_1}} g^{A,2,2}_{\gamma_{c_1},\alpha} \rangle\rangle \langle\langle g^{A,1,1}_{\alpha,\gamma_{c_2}} g^{A,2,2}_{\gamma_{c_2},\alpha} \rangle\rangle \tag{14}$$

$$= \frac{c_{1/2}}{16} \left(\frac{J_0}{W}\right)^{12} \frac{R_a}{l_e} \frac{1}{k_F R_{\alpha,\beta}} \frac{1}{k_F R_{\alpha,\gamma_{c,1}}} \frac{1}{k_F R_{\alpha,\gamma_{c,2}}} \frac{\Delta^6}{\left(\Delta^2 - (\omega - i\eta)^2\right)^3} \exp\left[i\left(-\varphi_a - \varphi_b + \varphi_{c_1} + \varphi_{c_2}\right)\right] \tag{15}$$

$$\langle\langle J_{(a,\alpha),(1,1)} G^{A,(-1,-1,1,1)}_{[12],(\alpha,a),(1,1),(1),3} \rangle\rangle = J_0^{12} \langle\langle g^{A,1,1}_{\alpha,\gamma_{c_1}} g^{A,1,1}_{c_1,c_1} g^{A,1,1}_{\gamma_{c_1},\gamma_{c_2}} g^{A,1,2}_{c_2,c_2} g^{A,2,2}_{\gamma_{c_2},\gamma_{c_1}} g^{A,2,2}_{c_1,c_1} g^{A,2,2}_{\gamma_{c_1},\beta} g^{A,2,1}_{b,b} g^{A,1,1}_{\beta,\gamma_{c_1}} g^{A,1,2}_{c_1,c_1} g^{A,2,2}_{\gamma_{c_1},\alpha} g^{A,2,1}_{a,a} \rangle\rangle \tag{16}$$

$$= J_0^{12} \langle\langle g^{A,2,1}_{a,a} \rangle\rangle \langle\langle g^{A,2,1}_{b,b} \rangle\rangle \langle\langle g^{A,1,1}_{c_1,c_1} g^{A,1,2}_{c_1,c_1} g^{A,2,2}_{c_1,c_1} \rangle\rangle \langle\langle g^{A,1,2}_{c_2,c_2} \rangle\rangle \langle\langle g^{A,1,1}_{\alpha,\gamma_{c_1}} g^{A,2,2}_{\gamma_{c_1},\alpha} \rangle\rangle \langle\langle g^{A,1,1}_{\beta,\gamma_{c_1}} g^{A,2,2}_{\gamma_{c_1},\beta} \rangle\rangle \langle\langle g^{A,1,1}_{\gamma_{c_1},\gamma_{c_2}} g^{A,2,2}_{\gamma_{c_2},\gamma_{c_1}} \rangle\rangle \tag{17}$$

$$= \frac{c_{1/2}}{16} \left(\frac{J_0}{W}\right)^{12} \frac{R_{c_1}}{l_e} \frac{1}{k_F R_{\alpha,\gamma_{c,1}}} \frac{1}{k_F R_{\beta,\gamma_{c,1}}} \frac{1}{k_F R_{\gamma_{c,1},\gamma_{c,2}}} \frac{\Delta^6}{\left(\Delta^2 - (\omega - i\eta)^2\right)^3} \exp\left[i\left(-\varphi_a - \varphi_b + \varphi_{c_1} + \varphi_{c_2}\right)\right] \tag{18}$$

$$\langle\langle J_{(a,\alpha),(1,1)} G^{A,(-1,-1,1,1)}_{[12],(\alpha,a),(1,1),(1),4}\rangle\rangle = J_0^{12}\langle\langle g^{A,1,1}_{\alpha,\gamma_{c_1}} g^{A,1,2}_{c_1,c_1} g^{A,2,2}_{\gamma_{c_1},\beta} g^{A,2,1}_{b,b} g^{A,1,1}_{\beta,\gamma_{c_1}} g^{A,1,1}_{c_1,c_1} g^{A,1,1}_{\gamma_{c_1},\gamma_{c_2}} g^{A,1,2}_{c_2,c_2} g^{A,2,2}_{\gamma_{c_2},\gamma_{c_1}} g^{A,2,2}_{c_1,c_1} g^{A,2,2}_{\gamma_{c_1},\alpha} g^{A,2,1}_{a,a}\rangle\rangle \tag{19}$$

$$= J_0^{12}\langle\langle g^{A,2,1}_{a,a}\rangle\rangle\langle\langle g^{A,2,1}_{b,b}\rangle\rangle\langle\langle g^{A,1,1}_{c_1,c_1} g^{A,1,2}_{c_1,c_1} g^{A,2,2}_{c_1,c_1}\rangle\rangle\langle\langle g^{A,1,2}_{c_2,c_2}\rangle\rangle\langle\langle g^{A,1,1}_{\alpha,\gamma_{c_1}} g^{A,2,2}_{\gamma_{c_1},\alpha}\rangle\rangle\langle\langle g^{A,1,1}_{\beta,\gamma_{c_1}} g^{A,2,2}_{\gamma_{c_1},\beta}\rangle\rangle\langle\langle g^{A,1,1}_{\gamma_{c_1},\gamma_{c_2}} g^{A,2,2}_{\gamma_{c_2},\gamma_{c_1}}\rangle\rangle \tag{20}$$

$$= \frac{c_{1/2}}{16}\left(\frac{J_0}{W}\right)^{12}\frac{R_{c_1}}{l_e}\frac{1}{k_F R_{\alpha,\gamma_{c,1}}}\frac{1}{k_F R_{\beta,\gamma_{c,1}}}\frac{1}{k_F R_{\gamma_{c,1},\gamma_{c,2}}}\frac{\Delta^6}{\left(\Delta^2-(\omega-i\eta)^2\right)^3}\exp\left[i\left(-\varphi_a-\varphi_b+\varphi_{c_1}+\varphi_{c_2}\right)\right] \tag{21}$$

$$\langle\langle J_{(a,\alpha),(1,1)} G^{A,(-1,-1,1,1)}_{[12],(\alpha,a),(1,1),(1),5}\rangle\rangle = J_0^{12}\langle\langle g^{A,1,1}_{\alpha,\gamma_{c_2}} g^{A,1,2}_{c_2,c_2} g^{A,2,2}_{\gamma_{c_2},\alpha} g^{A,2,1}_{a,a} g^{A,1,1}_{\alpha,\gamma_{c_1}} g^{A,1,2}_{c_1,c_1} g^{A,2,2}_{\gamma_{c_1},\alpha} g^{A,2,2}_{a,a} g^{A,2,2}_{\alpha,\beta} g^{A,2,1}_{b,b} g^{A,1,1}_{\beta,\alpha} g^{A,1,1}_{a,a}\rangle\rangle \tag{22}$$

$$= J_0^{12}\langle\langle g^{A,1,1}_{a,a} g^{A,2,1}_{a,a} g^{A,2,2}_{a,a}\rangle\rangle\langle\langle g^{A,2,1}_{b,b}\rangle\rangle\langle\langle g^{A,1,2}_{c_1,c_1}\rangle\rangle\langle\langle g^{A,1,2}_{c_2,c_2}\rangle\rangle\langle\langle g^{A,2,2}_{\alpha,\beta} g^{A,1,1}_{\beta,\alpha}\rangle\rangle\langle\langle g^{A,1,1}_{\alpha,\gamma_{c_1}} g^{A,2,2}_{\gamma_{c_1},\alpha}\rangle\rangle\langle\langle g^{A,1,1}_{\alpha,\gamma_{c_2}} g^{A,2,2}_{\gamma_{c_2},\alpha}\rangle\rangle \tag{23}$$

$$= \frac{c_{1/2}}{16}\left(\frac{J_0}{W}\right)^{12}\frac{R_a}{l_e}\frac{1}{k_F R_{\alpha,\beta}}\frac{1}{k_F R_{\alpha,\gamma_{c,1}}}\frac{1}{k_F R_{\alpha,\gamma_{c,2}}}\frac{\Delta^6}{\left(\Delta^2-(\omega-i\eta)^2\right)^3}\exp\left[i\left(-\varphi_a-\varphi_b+\varphi_{c_1}+\varphi_{c_2}\right)\right] \tag{24}$$

$$\langle\langle J_{(a,\alpha),(1,1)} G^{A,(-1,-1,1,1)}_{[12],(\alpha,a),(1,1),(1),6}\rangle\rangle = J_0^{12}\langle\langle g^{A,1,1}_{\alpha,\gamma_{c_2}} g^{A,1,2}_{c_2,c_2} g^{A,2,2}_{\gamma_{c_2},\alpha} g^{A,2,2}_{a,a} g^{A,2,2}_{\alpha,\beta} g^{A,2,1}_{b,b} g^{A,1,1}_{\beta,\alpha} g^{A,1,1}_{a,a} g^{A,1,1}_{\alpha,\gamma_{c_1}} g^{A,1,2}_{c_1,c_1} g^{A,2,2}_{\gamma_{c_1},\alpha} g^{A,2,1}_{a,a}\rangle\rangle \tag{25}$$

$$= J_0^{12}\langle\langle g^{A,1,1}_{a,a} g^{A,2,1}_{a,a} g^{A,2,2}_{a,a}\rangle\rangle\langle\langle g^{A,2,1}_{b,b}\rangle\rangle\langle\langle g^{A,1,2}_{c_1,c_1}\rangle\rangle\langle\langle g^{A,1,2}_{c_2,c_2}\rangle\rangle\langle\langle g^{A,2,2}_{\alpha,\beta} g^{A,1,1}_{\beta,\alpha}\rangle\rangle\langle\langle g^{A,1,1}_{\alpha,\gamma_{c_1}} g^{A,2,2}_{\gamma_{c_1},\alpha}\rangle\rangle\langle\langle g^{A,1,1}_{\alpha,\gamma_{c_2}} g^{A,2,2}_{\gamma_{c_2},\alpha}\rangle\rangle \tag{26}$$

$$= \frac{c_{1/2}}{16}\left(\frac{J_0}{W}\right)^{12}\frac{R_a}{l_e}\frac{1}{k_F R_{\alpha,\beta}}\frac{1}{k_F R_{\alpha,\gamma_{c,1}}}\frac{1}{k_F R_{\alpha,\gamma_{c,2}}}\frac{\Delta^6}{\left(\Delta^2-(\omega-i\eta)^2\right)^3}\exp\left[i\left(-\varphi_a-\varphi_b+\varphi_{c_1}+\varphi_{c_2}\right)\right] \tag{27}$$

$$\langle\langle J_{(a,\alpha),(1,1)} G^{A,(-1,-1,1,1)}_{[12],(\alpha,a),(1,1),(1),7}\rangle\rangle = J_0^{12}\langle\langle g^{A,1,1}_{\alpha,\gamma_{c_2}} g^{A,1,1}_{c_2,c_2} g^{A,1,1}_{\gamma_{c_2},\gamma_{c_1}} g^{A,1,2}_{c_1,c_1} g^{A,2,2}_{\gamma_{c_1},\gamma_{c_2}} g^{A,2,2}_{c_2,c_2} g^{A,2,2}_{\gamma_{c_2},\beta} g^{A,2,1}_{b,b} g^{A,1,1}_{\beta,\gamma_{c_2}} g^{A,1,2}_{c_2,c_2} g^{A,2,2}_{\gamma_{c_2},\alpha} g^{A,2,1}_{a,a}\rangle\rangle \tag{28}$$

$$= J_0^{12}\langle\langle g^{A,2,1}_{a,a}\rangle\rangle\langle\langle g^{A,2,1}_{b,b}\rangle\rangle\langle\langle g^{A,1,2}_{c_1,c_1}\rangle\rangle\langle\langle g^{A,1,1}_{c_2,c_2} g^{A,1,2}_{c_2,c_2} g^{A,2,2}_{c_2,c_2}\rangle\rangle\langle\langle g^{A,1,1}_{\alpha,\gamma_{c_2}} g^{A,2,2}_{\gamma_{c_2},\alpha}\rangle\rangle\langle\langle g^{A,1,1}_{\beta,\gamma_{c_2}} g^{A,2,2}_{\gamma_{c_2},\beta}\rangle\rangle\langle\langle g^{A,2,2}_{\gamma_{c_1},\gamma_{c_2}} g^{A,1,1}_{\gamma_{c_2},\gamma_{c_1}}\rangle\rangle \tag{29}$$

$$= \frac{c_{1/2}}{16}\left(\frac{J_0}{W}\right)^{12}\frac{R_{c_2}}{l_e}\frac{1}{k_F R_{\alpha,\gamma_{c,2}}}\frac{1}{k_F R_{\beta,\gamma_{c,2}}}\frac{1}{k_F R_{\gamma_{c,1},\gamma_{c,2}}}\frac{\Delta^6}{\left(\Delta^2-(\omega-i\eta)^2\right)^3}\exp\left[i\left(-\varphi_a-\varphi_b+\varphi_{c_1}+\varphi_{c_2}\right)\right] \tag{30}$$

$$\langle\langle J_{(a,\alpha),(1,1)} G^{A,(-1,-1,1,1)}_{[12],(\alpha,a),(1,1),(1),8}\rangle\rangle = J_0^{12}\langle\langle g^{A,1,1}_{\alpha,\gamma_{c_2}} g^{A,1,2}_{c_2,c_2} g^{A,2,2}_{\gamma_{c_2},\beta} g^{A,2,1}_{b,b} g^{A,1,1}_{\beta,\gamma_{c_2}} g^{A,1,1}_{c_2,c_2} g^{A,1,1}_{\gamma_{c_2},\gamma_{c_1}} g^{A,1,2}_{c_1,c_1} g^{A,2,2}_{\gamma_{c_1},\gamma_{c_2}} g^{A,2,2}_{c_2,c_2} g^{A,2,2}_{\gamma_{c_2},\alpha} g^{A,2,1}_{a,a}\rangle\rangle \tag{31}$$

$$= J_0^{12}\langle\langle g^{A,2,1}_{a,a}\rangle\rangle\langle\langle g^{A,2,1}_{b,b}\rangle\rangle\langle\langle g^{A,1,2}_{c_1,c_1}\rangle\rangle\langle\langle g^{A,1,1}_{c_2,c_2} g^{A,1,2}_{c_2,c_2} g^{A,2,2}_{c_2,c_2}\rangle\rangle\langle\langle g^{A,1,1}_{\alpha,\gamma_{c_2}} g^{A,2,2}_{\gamma_{c_2},\alpha}\rangle\rangle\langle\langle g^{A,1,1}_{\beta,\gamma_{c_2}} g^{A,2,2}_{\gamma_{c_2},\beta}\rangle\rangle\langle\langle g^{A,2,2}_{\gamma_{c_1},\gamma_{c_2}} g^{A,1,1}_{\gamma_{c_2},\gamma_{c_1}}\rangle\rangle \tag{32}$$

$$= \frac{c_{1/2}}{16}\left(\frac{J_0}{W}\right)^{12}\frac{R_{c_2}}{l_e}\frac{1}{k_F R_{\alpha,\gamma_{c,2}}}\frac{1}{k_F R_{\beta,\gamma_{c,2}}}\frac{1}{k_F R_{\gamma_{c,1},\gamma_{c,2}}}\frac{\Delta^6}{\left(\Delta^2-(\omega-i\eta)^2\right)^3}\exp\left[i\left(-\varphi_a-\varphi_b+\varphi_{c_1}+\varphi_{c_2}\right)\right] \tag{33}$$

$$\langle\langle J_{(a,\alpha),(1,1)} G^{A,(-1,-1,1,1)}_{[12],(\alpha,a),(1,1),(1),9}\rangle\rangle = J_0^{12}\langle\langle g^{A,1,1}_{\alpha,\beta} g^{A,1,1}_{b,b} g^{A,1,1}_{\beta,\gamma_{c_1}} g^{A,1,2}_{c_1,c_1} g^{A,2,2}_{\gamma_{c_1},\beta} g^{A,2,1}_{b,b} g^{A,1,1}_{\beta,\gamma_{c_2}} g^{A,1,2}_{c_2,c_2} g^{A,2,2}_{\gamma_{c_2},\beta} g^{A,2,2}_{b,b} g^{A,2,2}_{\beta,\alpha} g^{A,2,1}_{a,a}\rangle\rangle \tag{34}$$

$$= J_0^{12}\langle\langle g^{A,2,1}_{a,a}\rangle\rangle\langle\langle g^{A,1,1}_{b,b} g^{A,2,1}_{b,b} g^{A,2,2}_{b,b}\rangle\rangle\langle\langle g^{A,1,2}_{c_1,c_1}\rangle\rangle\langle\langle g^{A,1,2}_{c_2,c_2}\rangle\rangle\langle\langle g^{A,1,1}_{\alpha,\beta} g^{A,2,2}_{\beta,\alpha}\rangle\rangle\langle\langle g^{A,1,1}_{\beta,\gamma_{c_1}} g^{A,2,2}_{\gamma_{c_1},\beta}\rangle\rangle\langle\langle g^{A,1,1}_{\beta,\gamma_{c_2}} g^{A,2,2}_{\gamma_{c_2},\beta}\rangle\rangle \tag{35}$$

$$= \frac{c_{1/2}}{16}\left(\frac{J_0}{W}\right)^{12}\frac{R_b}{l_e}\frac{1}{k_F R_{\alpha,\beta}}\frac{1}{k_F R_{\beta,\gamma_{c,1}}}\frac{1}{k_F R_{\beta,\gamma_{c,2}}}\frac{\Delta^6}{\left(\Delta^2-(\omega-i\eta)^2\right)^3}\exp\left[i\left(-\varphi_a-\varphi_b+\varphi_{c_1}+\varphi_{c_2}\right)\right] \tag{36}$$

$$\langle\langle J_{(a,\alpha),(1,1)} G^{A,(-1,-1,1,1)}_{[12],(\alpha,a),(1,1),(1),10}\rangle\rangle = J_0^{12}\langle\langle g^{A,1,1}_{\alpha,\beta} g^{A,1,1}_{b,b} g^{A,1,1}_{\beta,\gamma_{c_2}} g^{A,1,2}_{c_2,c_2} g^{A,2,2}_{\gamma_{c_2},\beta} g^{A,2,1}_{b,b} g^{A,1,1}_{\beta,\gamma_{c_1}} g^{A,1,2}_{c_1,c_1} g^{A,2,2}_{\gamma_{c_1},\beta} g^{A,2,2}_{b,b} g^{A,2,2}_{\beta,\alpha} g^{A,2,1}_{a,a}\rangle\rangle \tag{37}$$

$$= J_0^{12}\langle\langle g^{A,2,1}_{a,a}\rangle\rangle\langle\langle g^{A,1,1}_{b,b} g^{A,2,1}_{b,b} g^{A,2,2}_{b,b}\rangle\rangle\langle\langle g^{A,1,2}_{c_1,c_1}\rangle\rangle\langle\langle g^{A,1,2}_{c_2,c_2}\rangle\rangle\langle\langle g^{A,1,1}_{\alpha,\beta} g^{A,2,2}_{\beta,\alpha}\rangle\rangle\langle\langle g^{A,1,1}_{\beta,\gamma_{c_1}} g^{A,2,2}_{\gamma_{c_1},\beta}\rangle\rangle\langle\langle g^{A,1,1}_{\beta,\gamma_{c_2}} g^{A,2,2}_{\gamma_{c_2},\beta}\rangle\rangle \tag{38}$$

$$= \frac{c_{1/2}}{16}\left(\frac{J_0}{W}\right)^{12}\frac{R_b}{l_e}\frac{1}{k_F R_{\alpha,\beta}}\frac{1}{k_F R_{\beta,\gamma_{c,1}}}\frac{1}{k_F R_{\beta,\gamma_{c,2}}}\frac{\Delta^6}{\left(\Delta^2-(\omega-i\eta)^2\right)^3}\exp\left[i\left(-\varphi_a-\varphi_b+\varphi_{c_1}+\varphi_{c_2}\right)\right] \tag{39}$$

### 2. *Spin-down hole/spin-down hole* $(2,2)$ *Nambu component*

We proceed further with detailing the two terms $\lambda = 1,2$ contributing to the "$(2,2)$" Nambu component, see Eq. (76) in the paper:

$$\langle\langle J_{(a,\alpha),(2,2)} G^{A,(-1,-1,1,1)}_{[12],(\alpha,a),(2,2),(1)}\rangle\rangle = \sum_{\lambda=1}^{2}\langle\langle J_{(a,\alpha),(2,2)} G^{A,(-1,-1,1,1)}_{[12],(\alpha,a),(2,2),(1),\lambda}\rangle\rangle. \tag{40}$$

$$\langle\langle J_{(a,\alpha),(2,2)} G^{A,(-1,-1,1,1)}_{[12],(\alpha,a),(2,2),(1),1} \rangle\rangle = J_0^{12} \langle\langle g^{A,2,2}_{\alpha,\beta} g^{A,2,1}_{b,b} g^{A,1,1}_{\beta,\alpha} g^{A,1,1}_{a,a} g^{A,1,1}_{\alpha,\gamma_{c_1}} g^{A,1,2}_{c_1,c_1} g^{A,2,2}_{\gamma_{c_1},\alpha} g^{A,2,1}_{a,a} g^{A,1,1}_{\alpha,\gamma_{c_2}} g^{A,1,2}_{c_2,c_2} g^{A,2,2}_{\gamma_{c_2},\alpha} g^{A,2,2}_{a,a} \rangle\rangle \tag{41}$$

$$= J_0^{12} \langle\langle g^{A,1,1}_{a,a} g^{A,2,1}_{a,a} g^{A,2,2}_{a,a} \rangle\rangle \langle\langle g^{A,2,1}_{b,b} \rangle\rangle \langle\langle g^{A,1,2}_{c_1,c_1} \rangle\rangle \langle\langle g^{A,1,2}_{c_2,c_2} \rangle\rangle \langle\langle g^{A,2,2}_{\alpha,\beta} g^{A,1,1}_{\beta,\alpha} \rangle\rangle \langle\langle g^{A,1,1}_{\alpha,\gamma_{c_1}} g^{A,2,2}_{\gamma_{c_1},\alpha} \rangle\rangle \langle\langle g^{A,1,1}_{\alpha,\gamma_{c_2}} g^{A,2,2}_{\gamma_{c_2},\alpha} \rangle\rangle \tag{42}$$

$$= \frac{c_{1/2}}{16} \left(\frac{J_0}{W}\right)^{12} \frac{R_a}{l_e} \frac{1}{k_F R_{\alpha,\beta}} \frac{1}{k_F R_{\alpha,\gamma_{c,1}}} \frac{1}{k_F R_{\alpha,\gamma_{c,2}}} \frac{\Delta^6}{\left(\Delta^2 - (\omega - i\eta)^2\right)^3} \exp\left[i\left(-\varphi_a - \varphi_b + \varphi_{c_1} + \varphi_{c_2}\right)\right] \tag{43}$$

$$\langle\langle J_{(a,\alpha),(2,2)} G^{A,(-1,-1,1,1)}_{[12],(\alpha,a),(2,2),(1),2} \rangle\rangle = J_0^{12} \langle\langle g^{A,2,2}_{\alpha,\beta} g^{A,2,1}_{b,b} g^{A,1,1}_{\beta,\alpha} g^{A,1,1}_{a,a} g^{A,1,1}_{\alpha,\gamma_{c_2}} g^{A,1,2}_{c_2,c_2} g^{A,2,2}_{\gamma_{c_2},\alpha} g^{A,2,1}_{a,a} g^{A,1,1}_{\alpha,\gamma_{c_1}} g^{A,1,2}_{c_1,c_1} g^{A,2,2}_{\gamma_{c_1},\alpha} g^{A,2,2}_{a,a} \rangle\rangle \tag{44}$$

$$= J_0^{12} \langle\langle g^{A,1,1}_{a,a} g^{A,2,1}_{a,a} g^{A,2,2}_{a,a} \rangle\rangle \langle\langle g^{A,2,1}_{b,b} \rangle\rangle \langle\langle g^{A,1,2}_{c_1,c_1} \rangle\rangle \langle\langle g^{A,1,2}_{c_2,c_2} \rangle\rangle \langle\langle g^{A,2,2}_{\alpha,\beta} g^{A,1,1}_{\beta,\alpha} \rangle\rangle \langle\langle g^{A,1,1}_{\alpha,\gamma_{c_1}} g^{A,2,2}_{\gamma_{c_1},\alpha} \rangle\rangle \langle\langle g^{A,1,1}_{\alpha,\gamma_{c_2}} g^{A,2,2}_{\gamma_{c_2},\alpha} \rangle\rangle \tag{45}$$

$$= \frac{c_{1/2}}{16} \left(\frac{J_0}{W}\right)^{12} \frac{R_a}{l_e} \frac{1}{k_F R_{\alpha,\beta}} \frac{1}{k_F R_{\alpha,\gamma_{c,1}}} \frac{1}{k_F R_{\alpha,\gamma_{c,2}}} \frac{\Delta^6}{\left(\Delta^2 - (\omega - i\eta)^2\right)^3} \exp\left[i\left(-\varphi_a - \varphi_b + \varphi_{c_1} + \varphi_{c_2}\right)\right] \tag{46}$$

## B. Evaluation of the leading order-$\mathscr{S}_{contact}/l_e^2$ contribution

Now, we consider the contributions appearing at the orders $(J_0/W)^{12}$ and $\mathscr{S}_{contact}/l_e^2$.

### 1. *Spin-up electron/spin-up electron* $(1,1)$ *Nambu component*

We first list the $\lambda = 1, ..., 20$ contributions to the $(1,1)$ Nambu component $\langle\langle J_{(a,\alpha),(1,1)} G^{A,(-1,-1,1,1)}_{[12],(\alpha,a),(1,1),(2)} \rangle\rangle$, see Eq. (80) in the paper:

$$\langle\langle J_{(a,\alpha),(1,1)} G^{A,(-1,-1,1,1)}_{[12],(\alpha,a),(1,1),(2)} \rangle\rangle = \sum_{\lambda=1}^{20} \langle\langle J_{(a,\alpha),(1,1)} G^{A,(-1,-1,1,1)}_{[12],(\alpha,a),(1,1),(2),\lambda} \rangle\rangle, \tag{47}$$

where the"$(2)$" label in the subscript refers to the considered terms of order $\mathscr{S}_{contact}/l_e^2$:

$$\langle\langle J_{(a,\alpha),(1,1)} G^{A,(-1,-1,1,1)}_{[12],(\alpha,a),(1,1),(2),1} \rangle\rangle = J_0^{12} \langle\langle g^{A,1,1}_{\alpha,\gamma_{c_1}} g^{A,1,2}_{c_1,c_1} g^{A,2,2}_{\gamma_{c_1},\alpha} g^{A,2,1}_{a,a} g^{A,1,1}_{\alpha,\gamma_{c_2}} g^{A,1,2}_{c_2,c_2} g^{A,2,2}_{\gamma_{c_2},\beta} g^{A,2,1}_{b,b} g^{A,1,1}_{\beta,\gamma_{c_2}} g^{A,1,1}_{c_2,c_2} g^{A,1,1}_{\gamma_{c_2},\alpha} g^{A,1,1}_{a,a} \rangle\rangle \tag{48}$$

$$= J_0^{12} \langle\langle g^{A,1,1}_{a,a} g^{A,2,1}_{a,a} \rangle\rangle \langle\langle g^{A,2,1}_{b,b} \rangle\rangle \langle\langle g^{A,1,2}_{c_1,c_1} \rangle\rangle \langle\langle g^{A,1,1}_{c_2,c_2} g^{A,1,2}_{c_2,c_2} \rangle\rangle \langle\langle g^{A,1,1}_{\alpha,\gamma_{c_1}} g^{A,2,2}_{\gamma_{c_1},\alpha} \rangle\rangle \langle\langle g^{A,1,1}_{\alpha,\gamma_{c_2}} g^{A,1,1}_{\gamma_{c_2},\alpha} \rangle\rangle \langle\langle g^{A,1,1}_{\beta,\gamma_{c_2}} g^{A,2,2}_{\gamma_{c_2},\beta} \rangle\rangle \tag{49}$$

$$= -\frac{c_1}{32} \left(\frac{J_0}{W}\right)^{12} \frac{R_a R_{c_2}}{(l_e)^2} \frac{1}{k_F R_{\alpha,\gamma_{c,1}}} \frac{1}{k_F R_{\alpha,\gamma_{c,2}}} \frac{1}{k_F R_{\beta,\gamma_{c,2}}} \frac{(\omega - i\eta)^2 \Delta^4}{\left(\Delta^2 - (\omega - i\eta)^2\right)^3} \exp\left[i\left(-\varphi_a - \varphi_b + \varphi_{c_1} + \varphi_{c_2}\right)\right] \tag{50}$$

$$\langle\langle J_{(a,\alpha),(1,1)} G^{A,(-1,-1,1,1)}_{[12],(\alpha,a),(1,1),(2),2} \rangle\rangle = J_0^{12} \langle\langle g^{A,1,1}_{\alpha,\gamma_{c_1}} g^{A,1,2}_{c_1,c_1} g^{A,2,2}_{\gamma_{c_1},\alpha} g^{A,2,2}_{a,a} g^{A,2,2}_{\alpha,\gamma_{c_2}} g^{A,2,2}_{c_2,c_2} g^{A,2,2}_{\gamma_{c_2},\beta} g^{A,2,1}_{b,b} g^{A,1,1}_{\beta,\gamma_{c_2}} g^{A,1,2}_{c_2,c_2} g^{A,2,2}_{\gamma_{c_2},\alpha} g^{A,2,1}_{a,a} \rangle\rangle \tag{51}$$

$$= J_0^{12} \langle\langle g^{A,2,1}_{a,a} g^{A,2,2}_{a,a} \rangle\rangle \langle\langle g^{A,2,1}_{b,b} \rangle\rangle \langle\langle g^{A,1,2}_{c_1,c_1} \rangle\rangle \langle\langle g^{A,1,2}_{c_2,c_2} g^{A,2,2}_{c_2,c_2} \rangle\rangle \langle\langle g^{A,1,1}_{\alpha,\gamma_{c_1}} g^{A,2,2}_{\gamma_{c_1},\alpha} \rangle\rangle \langle\langle g^{A,2,2}_{\alpha,\gamma_{c_2}} g^{A,2,2}_{\gamma_{c_2},\alpha} \rangle\rangle \langle\langle g^{A,1,1}_{\beta,\gamma_{c_2}} g^{A,2,2}_{\gamma_{c_2},\beta} \rangle\rangle \tag{52}$$

$$= -\frac{c_1}{32} \left(\frac{J_0}{W}\right)^{12} \frac{R_a R_{c_2}}{(l_e)^2} \frac{1}{k_F R_{\alpha,\gamma_{c,1}}} \frac{1}{k_F R_{\alpha,\gamma_{c,2}}} \frac{1}{k_F R_{\beta,\gamma_{c,2}}} \frac{(\omega - i\eta)^2 \Delta^4}{\left(\Delta^2 - (\omega - i\eta)^2\right)^3} \exp\left[i\left(-\varphi_a - \varphi_b + \varphi_{c_1} + \varphi_{c_2}\right)\right] \tag{53}$$

$$\langle\langle J_{(a,\alpha),(1,1)} G^{A,(-1,-1,1,1)}_{[12],(\alpha,a),(1,1),(2),3} \rangle\rangle = J_0^{12} \langle\langle g^{A,1,1}_{\alpha,\gamma_{c_1}} g^{A,1,2}_{c_1,c_1} g^{A,2,2}_{\gamma_{c_1},\alpha} g^{A,2,1}_{a,a} g^{A,1,1}_{\alpha,\beta} g^{A,1,1}_{b,b} g^{A,1,1}_{\beta,\gamma_{c_2}} g^{A,1,2}_{c_2,c_2} g^{A,2,2}_{\gamma_{c_2},\beta} g^{A,2,1}_{b,b} g^{A,1,1}_{\beta,\alpha} g^{A,1,1}_{a,a} \rangle\rangle \tag{54}$$

$$= J_0^{12} \langle\langle g^{A,1,1}_{a,a} g^{A,2,1}_{a,a} \rangle\rangle \langle\langle g^{A,1,1}_{b,b} g^{A,2,1}_{b,b} \rangle\rangle \langle\langle g^{A,1,2}_{c_1,c_1} \rangle\rangle \langle\langle g^{A,1,2}_{c_2,c_2} \rangle\rangle \langle\langle g^{A,1,1}_{\alpha,\beta} g^{A,1,1}_{\beta,\alpha} \rangle\rangle \langle\langle g^{A,1,1}_{\alpha,\gamma_{c_1}} g^{A,2,2}_{\gamma_{c_1},\alpha} \rangle\rangle \langle\langle g^{A,1,1}_{\beta,\gamma_{c_2}} g^{A,2,2}_{\gamma_{c_2},\beta} \rangle\rangle \tag{55}$$

$$= -\frac{c_1}{32} \left(\frac{J_0}{W}\right)^{12} \frac{R_a R_b}{(l_e)^2} \frac{1}{k_F R_{\alpha,\beta}} \frac{1}{k_F R_{\alpha,\gamma_{c,1}}} \frac{1}{k_F R_{\beta,\gamma_{c,2}}} \frac{(\omega - i\eta)^2 \Delta^4}{\left(\Delta^2 - (\omega - i\eta)^2\right)^3} \exp\left[i\left(-\varphi_a - \varphi_b + \varphi_{c_1} + \varphi_{c_2}\right)\right] \tag{56}$$

$$\langle\langle J_{(a,\alpha),(1,1)} G^{A,(-1,-1,1,1)}_{[12],(\alpha,a),(1,1),(2),4} \rangle\rangle = J_0^{12} \langle\langle g^{A,1,1}_{\alpha,\gamma_{c_1}} g^{A,1,2}_{c_1,c_1} g^{A,2,2}_{\gamma_{c_1},\alpha} g^{A,2,2}_{a,a} g^{A,2,2}_{\alpha,\beta} g^{A,2,1}_{b,b} g^{A,1,1}_{\beta,\gamma_{c_2}} g^{A,1,2}_{c_2,c_2} g^{A,2,2}_{\gamma_{c_2},\beta} g^{A,2,2}_{b,b} g^{A,2,2}_{\beta,\alpha} g^{A,2,1}_{a,a} \rangle\rangle \tag{57}$$

$$= J_0^{12} \langle\langle g^{A,2,1}_{a,a} g^{A,2,2}_{a,a} \rangle\rangle \langle\langle g^{A,2,1}_{b,b} g^{A,2,2}_{b,b} \rangle\rangle \langle\langle g^{A,1,2}_{c_1,c_1} \rangle\rangle \langle\langle g^{A,1,2}_{c_2,c_2} \rangle\rangle \langle\langle g^{A,2,2}_{\alpha,\beta} g^{A,2,2}_{\beta,\alpha} \rangle\rangle \langle\langle g^{A,1,1}_{\alpha,\gamma_{c_1}} g^{A,2,2}_{\gamma_{c_1},\alpha} \rangle\rangle \langle\langle g^{A,1,1}_{\beta,\gamma_{c_2}} g^{A,2,2}_{\gamma_{c_2},\beta} \rangle\rangle \tag{58}$$

$$= -\frac{c_1}{32} \left(\frac{J_0}{W}\right)^{12} \frac{R_a R_b}{(l_e)^2} \frac{1}{k_F R_{\alpha,\beta}} \frac{1}{k_F R_{\alpha,\gamma_{c,1}}} \frac{1}{k_F R_{\beta,\gamma_{c,2}}} \frac{(\omega - i\eta)^2 \Delta^4}{\left(\Delta^2 - (\omega - i\eta)^2\right)^3} \exp\left[i\left(-\varphi_a - \varphi_b + \varphi_{c_1} + \varphi_{c_2}\right)\right] \tag{59}$$

$$\langle\langle J_{(a,\alpha),(1,1)} G^{A,(-1,-1,1,1)}_{[12],(\alpha,a),(1,1),(2),5}\rangle\rangle = J_0^{12}\langle\langle g^{A,1,1}_{\alpha,\gamma_{c_1}} g^{A,1,2}_{c_1,c_1} g^{A,2,2}_{\gamma_{c_1},\gamma_{c_2}} g^{A,2,2}_{c_2,c_2} g^{A,2,2}_{\gamma_{c_2},\beta} g^{A,2,1}_{b,b} g^{A,1,1}_{\beta,\gamma_{c_2}} g^{A,1,2}_{c_2,c_2} g^{A,2,2}_{\gamma_{c_2},\gamma_{c_1}} g^{A,2,2}_{c_1,c_1} g^{A,2,2}_{\gamma_{c_1},\alpha} g^{A,2,1}_{a,a}\rangle\rangle \tag{60}$$

$$= J_0^{12}\langle\langle g^{A,2,1}_{a,a}\rangle\rangle\langle\langle g^{A,2,1}_{b,b}\rangle\rangle\langle\langle g^{A,1,2}_{c_1,c_1} g^{A,2,2}_{c_1,c_1}\rangle\rangle\langle\langle g^{A,1,2}_{c_2,c_2} g^{A,2,2}_{c_2,c_2}\rangle\rangle\langle\langle g^{A,1,1}_{\alpha,\gamma_{c_1}} g^{A,2,2}_{\gamma_{c_1},\alpha}\rangle\rangle\langle\langle g^{A,1,1}_{\beta,\gamma_{c_2}} g^{A,2,2}_{\gamma_{c_2},\beta}\rangle\rangle\langle\langle g^{A,2,2}_{\gamma_{c_1},\gamma_{c_2}} g^{A,2,2}_{\gamma_{c_2},\gamma_{c_1}}\rangle\rangle \tag{61}$$

$$= -\frac{c_1}{32}\left(\frac{J_0}{W}\right)^{12}\frac{R_{c_1}R_{c_2}}{(l_e)^2}\frac{1}{k_F R_{\alpha,\gamma_{c,1}}}\frac{1}{k_F R_{\beta,\gamma_{c,2}}}\frac{1}{k_F R_{\gamma_{c,1},\gamma_{c,2}}}\frac{(\omega-i\eta)^2\Delta^4}{\left(\Delta^2-(\omega-i\eta)^2\right)^3}\exp\left[i\left(-\varphi_a-\varphi_b+\varphi_{c_1}+\varphi_{c_2}\right)\right] \tag{62}$$

$$\langle\langle J_{(a,\alpha),(1,1)} G^{A,(-1,-1,1,1)}_{[12],(\alpha,a),(1,1),(2),6}\rangle\rangle = J_0^{12}\langle\langle g^{A,1,1}_{\alpha,\gamma_{c_1}} g^{A,1,1}_{c_1,c_1} g^{A,1,1}_{\gamma_{c_1},\gamma_{c_2}} g^{A,1,2}_{c_2,c_2} g^{A,2,2}_{\gamma_{c_2},\beta} g^{A,2,1}_{b,b} g^{A,1,1}_{\beta,\gamma_{c_2}} g^{A,1,1}_{c_2,c_2} g^{A,1,1}_{\gamma_{c_2},\gamma_{c_1}} g^{A,1,2}_{c_1,c_1} g^{A,2,2}_{\gamma_{c_1},\alpha} g^{A,2,1}_{a,a}\rangle\rangle \tag{63}$$

$$= J_0^{12}\langle\langle g^{A,2,1}_{a,a}\rangle\rangle\langle\langle g^{A,2,1}_{b,b}\rangle\rangle\langle\langle g^{A,1,1}_{c_1,c_1} g^{A,1,2}_{c_1,c_1}\rangle\rangle\langle\langle g^{A,1,1}_{c_2,c_2} g^{A,1,2}_{c_2,c_2}\rangle\rangle\langle\langle g^{A,1,1}_{\alpha,\gamma_{c_1}} g^{A,2,2}_{\gamma_{c_1},\alpha}\rangle\rangle\langle\langle g^{A,1,1}_{\beta,\gamma_{c_2}} g^{A,2,2}_{\gamma_{c_2},\beta}\rangle\rangle\langle\langle g^{A,1,1}_{\gamma_{c_1},\gamma_{c_2}} g^{A,1,1}_{\gamma_{c_2},\gamma_{c_1}}\rangle\rangle \tag{64}$$

$$= -\frac{c_1}{32}\left(\frac{J_0}{W}\right)^{12}\frac{R_{c_1}R_{c_2}}{(l_e)^2}\frac{1}{k_F R_{\alpha,\gamma_{c,1}}}\frac{1}{k_F R_{\beta,\gamma_{c,2}}}\frac{1}{k_F R_{\gamma_{c,1},\gamma_{c,2}}}\frac{(\omega-i\eta)^2\Delta^4}{\left(\Delta^2-(\omega-i\eta)^2\right)^3}\exp\left[i\left(-\varphi_a-\varphi_b+\varphi_{c_1}+\varphi_{c_2}\right)\right] \tag{65}$$

$$\langle\langle J_{(a,\alpha),(1,1)} G^{A,(-1,-1,1,1)}_{[12],(\alpha,a),(1,1),(2),7}\rangle\rangle = J_0^{12}\langle\langle g^{A,1,1}_{\alpha,\gamma_{c_1}} g^{A,1,2}_{c_1,c_1} g^{A,2,2}_{\gamma_{c_1},\beta} g^{A,2,1}_{b,b} g^{A,1,1}_{\beta,\gamma_{c_1}} g^{A,1,1}_{c_1,c_1} g^{A,1,1}_{\gamma_{c_1},\alpha} g^{A,1,1}_{a,a} g^{A,1,1}_{\alpha,\gamma_{c_2}} g^{A,1,2}_{c_2,c_2} g^{A,2,2}_{\gamma_{c_2},\alpha} g^{A,2,1}_{a,a}\rangle\rangle \tag{66}$$

$$= J_0^{12}\langle\langle g^{A,1,1}_{a,a} g^{A,2,1}_{a,a}\rangle\rangle\langle\langle g^{A,2,1}_{b,b}\rangle\rangle\langle\langle g^{A,1,1}_{c_1,c_1} g^{A,1,2}_{c_1,c_1}\rangle\rangle\langle\langle g^{A,1,2}_{c_2,c_2}\rangle\rangle\langle\langle g^{A,1,1}_{\alpha,\gamma_{c_1}} g^{A,1,1}_{\gamma_{c_1},\alpha}\rangle\rangle\langle\langle g^{A,1,1}_{\alpha,\gamma_{c_2}} g^{A,2,2}_{\gamma_{c_2},\alpha}\rangle\rangle\langle\langle g^{A,1,1}_{\beta,\gamma_{c_1}} g^{A,2,2}_{\gamma_{c_1},\beta}\rangle\rangle \tag{67}$$

$$= -\frac{c_1}{32}\left(\frac{J_0}{W}\right)^{12}\frac{R_aR_{c_1}}{(l_e)^2}\frac{1}{k_F R_{\alpha,\gamma_{c,1}}}\frac{1}{k_F R_{\alpha,\gamma_{c,2}}}\frac{1}{k_F R_{\beta,\gamma_{c,1}}}\frac{(\omega-i\eta)^2\Delta^4}{\left(\Delta^2-(\omega-i\eta)^2\right)^3}\exp\left[i\left(-\varphi_a-\varphi_b+\varphi_{c_1}+\varphi_{c_2}\right)\right] \tag{68}$$

$$\langle\langle J_{(a,\alpha),(1,1)} G^{A,(-1,-1,1,1)}_{[12],(\alpha,a),(1,1),(2),8}\rangle\rangle = J_0^{12}\langle\langle g^{A,1,1}_{\alpha,\gamma_{c_1}} g^{A,1,2}_{c_1,c_1} g^{A,2,2}_{\gamma_{c_1},\beta} g^{A,2,1}_{b,b} g^{A,1,1}_{\beta,\gamma_{c_2}} g^{A,1,2}_{c_2,c_2} g^{A,2,2}_{\gamma_{c_2},\beta} g^{A,2,2}_{b,b} g^{A,2,2}_{\beta,\gamma_{c_1}} g^{A,2,2}_{c_1,c_1} g^{A,2,2}_{\gamma_{c_1},\alpha} g^{A,2,1}_{a,a}\rangle\rangle \tag{69}$$

$$= J_0^{12}\langle\langle g^{A,2,1}_{a,a}\rangle\rangle\langle\langle g^{A,2,1}_{b,b} g^{A,2,2}_{b,b}\rangle\rangle\langle\langle g^{A,1,2}_{c_1,c_1} g^{A,2,2}_{c_1,c_1}\rangle\rangle\langle\langle g^{A,1,2}_{c_2,c_2}\rangle\rangle\langle\langle g^{A,1,1}_{\alpha,\gamma_{c_1}} g^{A,2,2}_{\gamma_{c_1},\alpha}\rangle\rangle\langle\langle g^{A,2,2}_{\beta,\gamma_{c_1}} g^{A,2,2}_{\gamma_{c_1},\beta}\rangle\rangle\langle\langle g^{A,1,1}_{\beta,\gamma_{c_2}} g^{A,2,2}_{\gamma_{c_2},\beta}\rangle\rangle \tag{70}$$

$$= -\frac{c_1}{32}\left(\frac{J_0}{W}\right)^{12}\frac{R_bR_{c_1}}{(l_e)^2}\frac{1}{k_F R_{\alpha,\gamma_{c,1}}}\frac{1}{k_F R_{\beta,\gamma_{c,1}}}\frac{1}{k_F R_{\beta,\gamma_{c,2}}}\frac{(\omega-i\eta)^2\Delta^4}{\left(\Delta^2-(\omega-i\eta)^2\right)^3}\exp\left[i\left(-\varphi_a-\varphi_b+\varphi_{c_1}+\varphi_{c_2}\right)\right] \tag{71}$$

$$\langle\langle J_{(a,\alpha),(1,1)} G^{A,(-1,-1,1,1)}_{[12],(\alpha,a),(1,1),(2),9}\rangle\rangle = J_0^{12}\langle\langle g^{A,1,1}_{\alpha,\gamma_{c_1}} g^{A,1,1}_{c_1,c_1} g^{A,1,1}_{\gamma_{c_1},\beta} g^{A,1,1}_{b,b} g^{A,1,1}_{\beta,\gamma_{c_2}} g^{A,1,2}_{c_2,c_2} g^{A,2,2}_{\gamma_{c_2},\beta} g^{A,2,1}_{b,b} g^{A,1,1}_{\beta,\gamma_{c_1}} g^{A,1,2}_{c_1,c_1} g^{A,2,2}_{\gamma_{c_1},\alpha} g^{A,2,1}_{a,a}\rangle\rangle \tag{72}$$

$$= J_0^{12}\langle\langle g^{A,2,1}_{a,a}\rangle\rangle\langle\langle g^{A,1,1}_{b,b} g^{A,2,1}_{b,b}\rangle\rangle\langle\langle g^{A,1,1}_{c_1,c_1} g^{A,1,2}_{c_1,c_1}\rangle\rangle\langle\langle g^{A,1,2}_{c_2,c_2}\rangle\rangle\langle\langle g^{A,1,1}_{\alpha,\gamma_{c_1}} g^{A,2,2}_{\gamma_{c_1},\alpha}\rangle\rangle\langle\langle g^{A,1,1}_{\beta,\gamma_{c_1}} g^{A,1,1}_{\gamma_{c_1},\beta}\rangle\rangle\langle\langle g^{A,1,1}_{\beta,\gamma_{c_2}} g^{A,2,2}_{\gamma_{c_2},\beta}\rangle\rangle \tag{73}$$

$$= -\frac{c_1}{32}\left(\frac{J_0}{W}\right)^{12}\frac{R_bR_{c_1}}{(l_e)^2}\frac{1}{k_F R_{\alpha,\gamma_{c,1}}}\frac{1}{k_F R_{\beta,\gamma_{c,1}}}\frac{1}{k_F R_{\beta,\gamma_{c,2}}}\frac{(\omega-i\eta)^2\Delta^4}{\left(\Delta^2-(\omega-i\eta)^2\right)^3}\exp\left[i\left(-\varphi_a-\varphi_b+\varphi_{c_1}+\varphi_{c_2}\right)\right] \tag{74}$$

$$\langle\langle J_{(a,\alpha),(1,1)} G^{A,(-1,-1,1,1)}_{[12],(\alpha,a),(1,1),(2),10}\rangle\rangle = J_0^{12}\langle\langle g^{A,1,1}_{\alpha,\gamma_{c_2}} g^{A,1,2}_{c_2,c_2} g^{A,2,2}_{\gamma_{c_2},\alpha} g^{A,2,1}_{a,a} g^{A,1,1}_{\alpha,\gamma_{c_1}} g^{A,1,2}_{c_1,c_1} g^{A,2,2}_{\gamma_{c_1},\beta} g^{A,2,1}_{b,b} g^{A,1,1}_{\beta,\gamma_{c_1}} g^{A,1,1}_{c_1,c_1} g^{A,1,1}_{\gamma_{c_1},\alpha} g^{A,1,1}_{a,a}\rangle\rangle \tag{75}$$

$$= J_0^{12}\langle\langle g^{A,1,1}_{a,a} g^{A,2,1}_{a,a}\rangle\rangle\langle\langle g^{A,2,1}_{b,b}\rangle\rangle\langle\langle g^{A,1,1}_{c_1,c_1} g^{A,1,2}_{c_1,c_1}\rangle\rangle\langle\langle g^{A,1,2}_{c_2,c_2}\rangle\rangle\langle\langle g^{A,1,1}_{\alpha,\gamma_{c_1}} g^{A,1,1}_{\gamma_{c_1},\alpha}\rangle\rangle\langle\langle g^{A,1,1}_{\alpha,\gamma_{c_2}} g^{A,2,2}_{\gamma_{c_2},\alpha}\rangle\rangle\langle\langle g^{A,1,1}_{\beta,\gamma_{c_1}} g^{A,2,2}_{\gamma_{c_1},\beta}\rangle\rangle \tag{76}$$

$$= -\frac{c_1}{32}\left(\frac{J_0}{W}\right)^{12}\frac{R_aR_{c_1}}{(l_e)^2}\frac{1}{k_F R_{\alpha,\gamma_{c,1}}}\frac{1}{k_F R_{\alpha,\gamma_{c,2}}}\frac{1}{k_F R_{\beta,\gamma_{c,1}}}\frac{(\omega-i\eta)^2\Delta^4}{\left(\Delta^2-(\omega-i\eta)^2\right)^3}\exp\left[i\left(-\varphi_a-\varphi_b+\varphi_{c_1}+\varphi_{c_2}\right)\right] \tag{77}$$

$$\langle\langle J_{(a,\alpha),(1,1)} G^{A,(-1,-1,1,1)}_{[12],(\alpha,a),(1,1),(2),11}\rangle\rangle = J_0^{12}\langle\langle g^{A,1,1}_{\alpha,\gamma_{c_2}} g^{A,1,2}_{c_2,c_2} g^{A,2,2}_{\gamma_{c_2},\alpha} g^{A,2,2}_{a,a} g^{A,2,2}_{\alpha,\gamma_{c_1}} g^{A,2,2}_{c_1,c_1} g^{A,2,2}_{\gamma_{c_1},\beta} g^{A,2,1}_{b,b} g^{A,1,1}_{\beta,\gamma_{c_1}} g^{A,1,2}_{c_1,c_1} g^{A,2,2}_{\gamma_{c_1},\alpha} g^{A,2,1}_{a,a}\rangle\rangle \tag{78}$$

$$= J_0^{12}\langle\langle g^{A,2,1}_{a,a} g^{A,2,2}_{a,a}\rangle\rangle\langle\langle g^{A,2,1}_{b,b}\rangle\rangle\langle\langle g^{A,1,2}_{c_1,c_1} g^{A,2,2}_{c_1,c_1}\rangle\rangle\langle\langle g^{A,1,2}_{c_2,c_2}\rangle\rangle\langle\langle g^{A,2,2}_{\alpha,\gamma_{c_1}} g^{A,2,2}_{\gamma_{c_1},\alpha}\rangle\rangle\langle\langle g^{A,1,1}_{\alpha,\gamma_{c_2}} g^{A,2,2}_{\gamma_{c_2},\alpha}\rangle\rangle\langle\langle g^{A,1,1}_{\beta,\gamma_{c_1}} g^{A,2,2}_{\gamma_{c_1},\beta}\rangle\rangle \tag{79}$$

$$= -\frac{c_1}{32}\left(\frac{J_0}{W}\right)^{12}\frac{R_aR_{c_1}}{(l_e)^2}\frac{1}{k_F R_{\alpha,\gamma_{c,1}}}\frac{1}{k_F R_{\alpha,\gamma_{c,2}}}\frac{1}{k_F R_{\beta,\gamma_{c,1}}}\frac{(\omega-i\eta)^2\Delta^4}{\left(\Delta^2-(\omega-i\eta)^2\right)^3}\exp\left[i\left(-\varphi_a-\varphi_b+\varphi_{c_1}+\varphi_{c_2}\right)\right] \tag{80}$$

$$\langle\langle J_{(a,\alpha),(1,1)} G^{A,(-1,-1,1,1)}_{[12],(\alpha,a),(1,1),(2),12}\rangle\rangle = J_0^{12}\langle\langle g^{A,1,1}_{\alpha,\gamma_{c_2}} g^{A,1,2}_{c_2,c_2} g^{A,2,2}_{\gamma_{c_2},\alpha} g^{A,2,1}_{a,a} g^{A,1,1}_{\alpha,\beta} g^{A,1,1}_{b,b} g^{A,1,1}_{\beta,\gamma_{c_1}} g^{A,1,2}_{c_1,c_1} g^{A,2,2}_{\gamma_{c_1},\beta} g^{A,2,1}_{b,b} g^{A,1,1}_{\beta,\alpha} g^{A,1,1}_{a,a}\rangle\rangle \tag{81}$$

$$= J_0^{12}\langle\langle g^{A,1,1}_{a,a} g^{A,2,1}_{a,a}\rangle\rangle\langle\langle g^{A,1,1}_{b,b} g^{A,2,1}_{b,b}\rangle\rangle\langle\langle g^{A,1,2}_{c_1,c_1}\rangle\rangle\langle\langle g^{A,1,2}_{c_2,c_2}\rangle\rangle\langle\langle g^{A,1,1}_{\alpha,\beta} g^{A,1,1}_{\beta,\alpha}\rangle\rangle\langle\langle g^{A,1,1}_{\alpha,\gamma_{c_2}} g^{A,2,2}_{\gamma_{c_2},\alpha}\rangle\rangle\langle\langle g^{A,1,1}_{\beta,\gamma_{c_1}} g^{A,2,2}_{\gamma_{c_1},\beta}\rangle\rangle \tag{82}$$

$$= -\frac{c_1}{32}\left(\frac{J_0}{W}\right)^{12}\frac{R_aR_b}{(l_e)^2}\frac{1}{k_F R_{\alpha,\beta}}\frac{1}{k_F R_{\alpha,\gamma_{c,2}}}\frac{1}{k_F R_{\beta,\gamma_{c,1}}}\frac{(\omega-i\eta)^2\Delta^4}{\left(\Delta^2-(\omega-i\eta)^2\right)^3}\exp\left[i\left(-\varphi_a-\varphi_b+\varphi_{c_1}+\varphi_{c_2}\right)\right] \tag{83}$$

$$\langle\langle J_{(a,\alpha),(1,1)} G^{A,(-1,-1,1,1)}_{[12],(\alpha,a),(1,1),(2),13}\rangle\rangle = J_0^{12}\langle\langle g^{A,1,1}_{\alpha,\gamma_{c_2}} g^{A,1,2}_{c_2,c_2} g^{A,2,2}_{\gamma_{c_2},\alpha} g^{A,2,2}_{a,a} g^{A,2,2}_{\alpha,\beta} g^{A,2,1}_{b,b} g^{A,1,1}_{\beta,\gamma_{c_1}} g^{A,1,2}_{c_1,c_1} g^{A,2,2}_{\gamma_{c_1},\beta} g^{A,2,2}_{b,b} g^{A,2,2}_{\beta,\alpha} g^{A,2,1}_{a,a}\rangle\rangle \tag{84}$$

$$= J_0^{12}\langle\langle g^{A,2,1}_{a,a} g^{A,2,2}_{a,a}\rangle\rangle\langle\langle g^{A,2,1}_{b,b} g^{A,2,2}_{b,b}\rangle\rangle\langle\langle g^{A,1,2}_{c_1,c_1}\rangle\rangle\langle\langle g^{A,1,2}_{c_2,c_2}\rangle\rangle\langle\langle g^{A,2,2}_{\alpha,\beta} g^{A,2,2}_{\beta,\alpha}\rangle\rangle\langle\langle g^{A,1,1}_{\alpha,\gamma_{c_2}} g^{A,2,2}_{\gamma_{c_2},\alpha}\rangle\rangle\langle\langle g^{A,1,1}_{\beta,\gamma_{c_1}} g^{A,2,2}_{\gamma_{c_1},\beta}\rangle\rangle \tag{85}$$

$$= -\frac{c_1}{32}\left(\frac{J_0}{W}\right)^{12}\frac{R_aR_b}{(l_e)^2}\frac{1}{k_F R_{\alpha,\beta}}\frac{1}{k_F R_{\alpha,\gamma_{c,2}}}\frac{1}{k_F R_{\beta,\gamma_{c,1}}}\frac{(\omega-i\eta)^2\Delta^4}{\left(\Delta^2-(\omega-i\eta)^2\right)^3}\exp\left[i\left(-\varphi_a-\varphi_b+\varphi_{c_1}+\varphi_{c_2}\right)\right] \tag{86}$$

$$\langle\langle J_{(a,\alpha),(1,1)} G^{A,(-1,-1,1,1)}_{[12],(\alpha,a),(1,1),(2),14}\rangle\rangle = J_0^{12}\langle\langle g^{A,1,1}_{\alpha,\gamma_{c_2}} g^{A,1,2}_{c_2,c_2} g^{A,2,2}_{\gamma_{c_2},\gamma_{c_1}} g^{A,2,2}_{c_1,c_1} g^{A,2,2}_{\gamma_{c_1},\beta} g^{A,2,1}_{b,b} g^{A,1,1}_{\beta,\gamma_{c_1}} g^{A,1,2}_{c_1,c_1} g^{A,2,2}_{\gamma_{c_1},\gamma_{c_2}} g^{A,2,2}_{c_2,c_2} g^{A,2,2}_{\gamma_{c_2},\alpha} g^{A,2,1}_{a,a}\rangle\rangle \tag{87}$$

$$= J_0^{12}\langle\langle g^{A,2,1}_{a,a}\rangle\rangle\langle\langle g^{A,2,1}_{b,b}\rangle\rangle\langle\langle g^{A,1,2}_{c_1,c_1} g^{A,2,2}_{c_1,c_1}\rangle\rangle\langle\langle g^{A,1,2}_{c_2,c_2} g^{A,2,2}_{c_2,c_2}\rangle\rangle\langle\langle g^{A,1,1}_{\alpha,\gamma_{c_2}} g^{A,2,2}_{\gamma_{c_2},\alpha}\rangle\rangle\langle\langle g^{A,1,1}_{\beta,\gamma_{c_1}} g^{A,2,2}_{\gamma_{c_1},\beta}\rangle\rangle\langle\langle g^{A,2,2}_{\gamma_{c_1},\gamma_{c_2}} g^{A,2,2}_{\gamma_{c_2},\gamma_{c_1}}\rangle\rangle \tag{88}$$

$$= -\frac{c_1}{32}\left(\frac{J_0}{W}\right)^{12}\frac{R_{c_1}R_{c_2}}{(l_e)^2}\frac{1}{k_F R_{\alpha,\gamma_{c,2}}}\frac{1}{k_F R_{\beta,\gamma_{c,1}}}\frac{1}{k_F R_{\gamma_{c,1},\gamma_{c,2}}}\frac{(\omega-i\eta)^2\Delta^4}{\left(\Delta^2-(\omega-i\eta)^2\right)^3}\exp\left[i\left(-\varphi_a-\varphi_b+\varphi_{c_1}+\varphi_{c_2}\right)\right] \tag{89}$$

$$\langle\langle J_{(a,\alpha),(1,1)} G^{A,(-1,-1,1,1)}_{[12],(\alpha,a),(1,1),(2),15}\rangle\rangle = J_0^{12}\langle\langle g^{A,1,1}_{\alpha,\gamma_{c_2}} g^{A,1,1}_{c_2,c_2} g^{A,1,1}_{\gamma_{c_2},\gamma_{c_1}} g^{A,1,2}_{c_1,c_1} g^{A,2,2}_{\gamma_{c_1},\beta} g^{A,2,1}_{b,b} g^{A,1,1}_{\beta,\gamma_{c_1}} g^{A,1,1}_{c_1,c_1} g^{A,1,1}_{\gamma_{c_1},\gamma_{c_2}} g^{A,1,2}_{c_2,c_2} g^{A,2,2}_{\gamma_{c_2},\alpha} g^{A,2,1}_{a,a}\rangle\rangle \tag{90}$$

$$= J_0^{12}\langle\langle g^{A,2,1}_{a,a}\rangle\rangle\langle\langle g^{A,2,1}_{b,b}\rangle\rangle\langle\langle g^{A,1,1}_{c_1,c_1} g^{A,1,2}_{c_1,c_1}\rangle\rangle\langle\langle g^{A,1,1}_{c_2,c_2} g^{A,1,2}_{c_2,c_2}\rangle\rangle\langle\langle g^{A,1,1}_{\alpha,\gamma_{c_2}} g^{A,2,2}_{\gamma_{c_2},\alpha}\rangle\rangle\langle\langle g^{A,1,1}_{\beta,\gamma_{c_1}} g^{A,2,2}_{\gamma_{c_1},\beta}\rangle\rangle\langle\langle g^{A,1,1}_{\gamma_{c_1},\gamma_{c_2}} g^{A,1,1}_{\gamma_{c_2},\gamma_{c_1}}\rangle\rangle \tag{91}$$

$$= -\frac{c_1}{32}\left(\frac{J_0}{W}\right)^{12}\frac{R_{c_1}R_{c_2}}{(l_e)^2}\frac{1}{k_F R_{\alpha,\gamma_{c,2}}}\frac{1}{k_F R_{\beta,\gamma_{c,1}}}\frac{1}{k_F R_{\gamma_{c,1},\gamma_{c,2}}}\frac{(\omega-i\eta)^2\Delta^4}{\left(\Delta^2-(\omega-i\eta)^2\right)^3}\exp\left[i\left(-\varphi_a-\varphi_b+\varphi_{c_1}+\varphi_{c_2}\right)\right] \tag{92}$$

$$\langle\langle J_{(a,\alpha),(1,1)} G^{A,(-1,-1,1,1)}_{[12],(\alpha,a),(1,1),(2),16}\rangle\rangle = J_0^{12}\langle\langle g^{A,1,1}_{\alpha,\gamma_{c_2}} g^{A,1,2}_{c_2,c_2} g^{A,2,2}_{\gamma_{c_2},\beta} g^{A,2,1}_{b,b} g^{A,1,1}_{\beta,\gamma_{c_1}} g^{A,1,2}_{c_1,c_1} g^{A,2,2}_{\gamma_{c_1},\beta} g^{A,2,2}_{b,b} g^{A,2,2}_{\beta,\gamma_{c_2}} g^{A,2,2}_{c_2,c_2} g^{A,2,2}_{\gamma_{c_2},\alpha} g^{A,2,1}_{a,a}\rangle\rangle \tag{93}$$

$$= J_0^{12}\langle\langle g^{A,2,1}_{a,a}\rangle\rangle\langle\langle g^{A,2,1}_{b,b} g^{A,2,2}_{b,b}\rangle\rangle\langle\langle g^{A,1,2}_{c_1,c_1}\rangle\rangle\langle\langle g^{A,1,2}_{c_2,c_2} g^{A,2,2}_{c_2,c_2}\rangle\rangle\langle\langle g^{A,1,1}_{\alpha,\gamma_{c_2}} g^{A,2,2}_{\gamma_{c_2},\alpha}\rangle\rangle\langle\langle g^{A,1,1}_{\beta,\gamma_{c_1}} g^{A,2,2}_{\gamma_{c_1},\beta}\rangle\rangle\langle\langle g^{A,2,2}_{\beta,\gamma_{c_2}} g^{A,2,2}_{\gamma_{c_2},\beta}\rangle\rangle \tag{94}$$

$$= -\frac{c_1}{32}\left(\frac{J_0}{W}\right)^{12}\frac{R_b R_{c_2}}{(l_e)^2}\frac{1}{k_F R_{\alpha,\gamma_{c,2}}}\frac{1}{k_F R_{\beta,\gamma_{c,1}}}\frac{1}{k_F R_{\beta,\gamma_{c,2}}}\frac{(\omega-i\eta)^2\Delta^4}{\left(\Delta^2-(\omega-i\eta)^2\right)^3}\exp\left[i\left(-\varphi_a-\varphi_b+\varphi_{c_1}+\varphi_{c_2}\right)\right] \tag{95}$$

$$\langle\langle J_{(a,\alpha),(1,1)} G^{A,(-1,-1,1,1)}_{[12],(\alpha,a),(1,1),(2),17}\rangle\rangle = J_0^{12}\langle\langle g^{A,1,1}_{\alpha,\gamma_{c_2}} g^{A,1,1}_{c_2,c_2} g^{A,1,1}_{\gamma_{c_2},\beta} g^{A,1,1}_{b,b} g^{A,1,1}_{\beta,\gamma_{c_1}} g^{A,1,2}_{c_1,c_1} g^{A,2,2}_{\gamma_{c_1},\beta} g^{A,2,1}_{b,b} g^{A,1,1}_{\beta,\gamma_{c_2}} g^{A,1,2}_{c_2,c_2} g^{A,2,2}_{\gamma_{c_2},\alpha} g^{A,2,1}_{a,a}\rangle\rangle \tag{96}$$

$$= J_0^{12}\langle\langle g^{A,2,1}_{a,a}\rangle\rangle\langle\langle g^{A,1,1}_{b,b} g^{A,2,1}_{b,b}\rangle\rangle\langle\langle g^{A,1,2}_{c_1,c_1}\rangle\rangle\langle\langle g^{A,1,1}_{c_2,c_2} g^{A,1,2}_{c_2,c_2}\rangle\rangle\langle\langle g^{A,1,1}_{\alpha,\gamma_{c_2}} g^{A,2,2}_{\gamma_{c_2},\alpha}\rangle\rangle\langle\langle g^{A,1,1}_{\beta,\gamma_{c_1}} g^{A,2,2}_{\gamma_{c_1},\beta}\rangle\rangle\langle\langle g^{A,1,1}_{\beta,\gamma_{c_2}} g^{A,1,1}_{\gamma_{c_2},\beta}\rangle\rangle \tag{97}$$

$$= -\frac{c_1}{32}\left(\frac{J_0}{W}\right)^{12}\frac{R_b R_{c_2}}{(l_e)^2}\frac{1}{k_F R_{\alpha,\gamma_{c,2}}}\frac{1}{k_F R_{\beta,\gamma_{c,1}}}\frac{1}{k_F R_{\beta,\gamma_{c,2}}}\frac{(\omega-i\eta)^2\Delta^4}{\left(\Delta^2-(\omega-i\eta)^2\right)^3}\exp\left[i\left(-\varphi_a-\varphi_b+\varphi_{c_1}+\varphi_{c_2}\right)\right] \tag{98}$$

$$\langle\langle J_{(a,\alpha),(1,1)} G^{A,(-1,-1,1,1)}_{[12],(\alpha,a),(1,1),(2),18}\rangle\rangle = J_0^{12}\langle\langle g^{A,1,1}_{\alpha,\gamma_{c_2}} g^{A,1,2}_{c_2,c_2} g^{A,2,2}_{\gamma_{c_2},\beta} g^{A,2,1}_{b,b} g^{A,1,1}_{\beta,\gamma_{c_2}} g^{A,1,1}_{c_2,c_2} g^{A,1,1}_{\gamma_{c_2},\alpha} g^{A,1,1}_{a,a} g^{A,1,1}_{\alpha,\gamma_{c_1}} g^{A,1,2}_{c_1,c_1} g^{A,2,2}_{\gamma_{c_1},\alpha} g^{A,2,1}_{a,a}\rangle\rangle \tag{99}$$

$$= J_0^{12}\langle\langle g^{A,1,1}_{a,a} g^{A,2,1}_{a,a}\rangle\rangle\langle\langle g^{A,2,1}_{b,b}\rangle\rangle\langle\langle g^{A,1,2}_{c_1,c_1}\rangle\rangle\langle\langle g^{A,1,1}_{c_2,c_2} g^{A,1,2}_{c_2,c_2}\rangle\rangle\langle\langle g^{A,1,1}_{\alpha,\gamma_{c_1}} g^{A,2,2}_{\gamma_{c_1},\alpha}\rangle\rangle\langle\langle g^{A,1,1}_{\alpha,\gamma_{c_2}} g^{A,1,1}_{\gamma_{c_2},\alpha}\rangle\rangle\langle\langle g^{A,1,1}_{\beta,\gamma_{c_2}} g^{A,2,2}_{\gamma_{c_2},\beta}\rangle\rangle \tag{100}$$

$$= -\frac{c_1}{32}\left(\frac{J_0}{W}\right)^{12}\frac{R_a R_{c_2}}{(l_e)^2}\frac{1}{k_F R_{\alpha,\gamma_{c,1}}}\frac{1}{k_F R_{\alpha,\gamma_{c,2}}}\frac{1}{k_F R_{\beta,\gamma_{c,2}}}\frac{(\omega-i\eta)^2\Delta^4}{\left(\Delta^2-(\omega-i\eta)^2\right)^3}\exp\left[i\left(-\varphi_a-\varphi_b+\varphi_{c_1}+\varphi_{c_2}\right)\right] \tag{101}$$

$$\langle\langle J_{(a,\alpha),(1,1)} G^{A,(-1,-1,1,1)}_{[12],(\alpha,a),(1,1),(2),19}\rangle\rangle = J_0^{12}\langle\langle g^{A,1,1}_{\alpha,\beta} g^{A,1,1}_{b,b} g^{A,1,1}_{\beta,\gamma_{c_1}} g^{A,1,2}_{c_1,c_1} g^{A,2,2}_{\gamma_{c_1},\beta} g^{A,2,1}_{b,b} g^{A,1,1}_{\beta,\alpha} g^{A,1,1}_{a,a} g^{A,1,1}_{\alpha,\gamma_{c_2}} g^{A,1,2}_{c_2,c_2} g^{A,2,2}_{\gamma_{c_2},\alpha} g^{A,2,1}_{a,a}\rangle\rangle \tag{102}$$

$$= J_0^{12}\langle\langle g^{A,1,1}_{a,a} g^{A,2,1}_{a,a}\rangle\rangle\langle\langle g^{A,1,1}_{b,b} g^{A,2,1}_{b,b}\rangle\rangle\langle\langle g^{A,1,2}_{c_1,c_1}\rangle\rangle\langle\langle g^{A,1,2}_{c_2,c_2}\rangle\rangle\langle\langle g^{A,1,1}_{\alpha,\beta} g^{A,1,1}_{\beta,\alpha}\rangle\rangle\langle\langle g^{A,1,1}_{\alpha,\gamma_{c_2}} g^{A,2,2}_{\gamma_{c_2},\alpha}\rangle\rangle\langle\langle g^{A,1,1}_{\beta,\gamma_{c_1}} g^{A,2,2}_{\gamma_{c_1},\beta}\rangle\rangle \tag{103}$$

$$= -\frac{c_1}{32}\left(\frac{J_0}{W}\right)^{12}\frac{R_a R_b}{(l_e)^2}\frac{1}{k_F R_{\alpha,\beta}}\frac{1}{k_F R_{\alpha,\gamma_{c,2}}}\frac{1}{k_F R_{\beta,\gamma_{c,1}}}\frac{(\omega-i\eta)^2\Delta^4}{\left(\Delta^2-(\omega-i\eta)^2\right)^3}\exp\left[i\left(-\varphi_a-\varphi_b+\varphi_{c_1}+\varphi_{c_2}\right)\right] \tag{104}$$

$$\langle\langle J_{(a,\alpha),(1,1)} G^{A,(-1,-1,1,1)}_{[12],(\alpha,a),(1,1),(2),20}\rangle\rangle = J_0^{12}\langle\langle g^{A,1,1}_{\alpha,\beta} g^{A,1,1}_{b,b} g^{A,1,1}_{\beta,\gamma_{c_2}} g^{A,1,2}_{c_2,c_2} g^{A,2,2}_{\gamma_{c_2},\beta} g^{A,2,1}_{b,b} g^{A,1,1}_{\beta,\alpha} g^{A,1,1}_{a,a} g^{A,1,1}_{\alpha,\gamma_{c_1}} g^{A,1,2}_{c_1,c_1} g^{A,2,2}_{\gamma_{c_1},\alpha} g^{A,2,1}_{a,a}\rangle\rangle \tag{105}$$

$$= J_0^{12}\langle\langle g^{A,1,1}_{a,a} g^{A,2,1}_{a,a}\rangle\rangle\langle\langle g^{A,1,1}_{b,b} g^{A,2,1}_{b,b}\rangle\rangle\langle\langle g^{A,1,2}_{c_1,c_1}\rangle\rangle\langle\langle g^{A,1,2}_{c_2,c_2}\rangle\rangle\langle\langle g^{A,1,1}_{\alpha,\beta} g^{A,1,1}_{\beta,\alpha}\rangle\rangle\langle\langle g^{A,1,1}_{\alpha,\gamma_{c_1}} g^{A,2,2}_{\gamma_{c_1},\alpha}\rangle\rangle\langle\langle g^{A,1,1}_{\beta,\gamma_{c_2}} g^{A,2,2}_{\gamma_{c_2},\beta}\rangle\rangle \tag{106}$$

$$= -\frac{c_1}{32}\left(\frac{J_0}{W}\right)^{12}\frac{R_a R_b}{(l_e)^2}\frac{1}{k_F R_{\alpha,\beta}}\frac{1}{k_F R_{\alpha,\gamma_{c,1}}}\frac{1}{k_F R_{\beta,\gamma_{c,2}}}\frac{(\omega-i\eta)^2\Delta^4}{\left(\Delta^2-(\omega-i\eta)^2\right)^3}\exp\left[i\left(-\varphi_a-\varphi_b+\varphi_{c_1}+\varphi_{c_2}\right)\right] \tag{107}$$

### 2. *Spin-down hole/spin-down hole* $(2,2)$ *Nambu component*

Finally, we list the $\lambda = 1,...,4$ contributions to the $(2,2)$ Nambu component $\langle\langle J_{(a,\alpha),(2,2)} G^{A,(-1,-1,1,1)}_{[12],(\alpha,a),(2,2),(2)}\rangle\rangle$, see Eq. (82) in the paper:

$$\langle\langle J_{(a,\alpha),(2,2)} G^{A,(-1,-1,1,1)}_{[12],(\alpha,a),(2,2),(2)}\rangle\rangle = \sum_{\lambda=1}^{4}\langle\langle J_{(a,\alpha),(2,2)} G^{A,(-1,-1,1,1)}_{[12],(\alpha,a),(2,2),(2),\lambda}\rangle\rangle. \tag{108}$$

$$\langle\langle J_{(a,\alpha),(2,2)} G^{A,(-1,-1,1,1)}_{[12],(\alpha,a),(2,2),(2),1}\rangle\rangle = J_0^{12}\langle\langle g^{A,2,2}_{\alpha,\gamma_{c_1}} g^{A,2,2}_{c_1,c_1} g^{A,2,2}_{\gamma_{c_1},\beta} g^{A,2,1}_{b,b} g^{A,1,1}_{\beta,\gamma_{c_1}} g^{A,1,2}_{c_1,c_1} g^{A,2,2}_{\gamma_{c_1},\alpha} g^{A,2,1}_{a,a} g^{A,1,1}_{\alpha,\gamma_{c_2}} g^{A,1,2}_{c_2,c_2} g^{A,2,2}_{\gamma_{c_2},\alpha} g^{A,2,2}_{a,a}\rangle\rangle \tag{109}$$

$$= J_0^{12}\langle\langle g^{A,2,1}_{a,a} g^{A,2,2}_{a,a}\rangle\rangle\langle\langle g^{A,2,1}_{b,b}\rangle\rangle\langle\langle g^{A,1,2}_{c_1,c_1} g^{A,2,2}_{c_1,c_1}\rangle\rangle\langle\langle g^{A,1,2}_{c_2,c_2}\rangle\rangle\langle\langle g^{A,2,2}_{\alpha,\gamma_{c_1}} g^{A,2,2}_{\gamma_{c_1},\alpha}\rangle\rangle\langle\langle g^{A,1,1}_{\alpha,\gamma_{c_2}} g^{A,2,2}_{\gamma_{c_2},\alpha}\rangle\rangle\langle\langle g^{A,1,1}_{\beta,\gamma_{c_1}} g^{A,2,2}_{\gamma_{c_1},\beta}\rangle\rangle \tag{110}$$

$$= -\frac{c_1}{32}\left(\frac{J_0}{W}\right)^{12}\frac{R_a R_{c_1}}{(l_e)^2}\frac{1}{k_F R_{\alpha,\gamma_{c,1}}}\frac{1}{k_F R_{\alpha,\gamma_{c,2}}}\frac{1}{k_F R_{\beta,\gamma_{c,1}}}\frac{(\omega-i\eta)^2\Delta^4}{\left(\Delta^2-(\omega-i\eta)^2\right)^3}\exp\left[i\left(-\varphi_a-\varphi_b+\varphi_{c_1}+\varphi_{c_2}\right)\right] \tag{111}$$

$$\langle\langle J_{(a,\alpha),(2,2)} G^{A,(-1,-1,1,1)}_{[12],(\alpha,a),(2,2),(2),2} \rangle\rangle = J_0^{12} \langle\langle g^{A,2,2}_{\alpha,\gamma_{c_2}} g^{A,2,2}_{c_2,c_2} g^{A,2,2}_{\gamma_{c_2},\beta} g^{A,2,1}_{b,b} g^{A,1,1}_{\beta,\gamma_{c_2}} g^{A,1,2}_{c_2,c_2} g^{A,2,2}_{\gamma_{c_2},\alpha} g^{A,2,1}_{a,a} g^{A,1,1}_{\alpha,\gamma_{c_1}} g^{A,1,2}_{c_1,c_1} g^{A,2,2}_{\gamma_{c_1},\alpha} g^{A,2,2}_{a,a} \rangle\rangle \tag{112}$$

$$= J_0^{12} \langle\langle g^{A,2,1}_{a,a} g^{A,2,2}_{a,a} \rangle\rangle \langle\langle g^{A,2,1}_{b,b} \rangle\rangle \langle\langle g^{A,1,2}_{c_1,c_1} \rangle\rangle \langle\langle g^{A,1,2}_{c_2,c_2} g^{A,2,2}_{c_2,c_2} \rangle\rangle \langle\langle g^{A,1,1}_{\alpha,\gamma_{c_1}} g^{A,2,2}_{\gamma_{c_1},\alpha} \rangle\rangle \langle\langle g^{A,2,2}_{\alpha,\gamma_{c_2}} g^{A,2,2}_{\gamma_{c_2},\alpha} \rangle\rangle \langle\langle g^{A,1,1}_{\beta,\gamma_{c_2}} g^{A,2,2}_{\gamma_{c_2},\beta} \rangle\rangle \tag{113}$$

$$= -\frac{c_1}{32} \left(\frac{J_0}{W}\right)^{12} \frac{R_a R_{c_2}}{(l_e)^2} \frac{1}{k_F R_{\alpha,\gamma_{c,1}}} \frac{1}{k_F R_{\alpha,\gamma_{c,2}}} \frac{1}{k_F R_{\beta,\gamma_{c,2}}} \frac{(\omega - i\eta)^2 \Delta^4}{\left(\Delta^2 - (\omega - i\eta)^2\right)^3} \exp\left[i\left(-\varphi_a - \varphi_b + \varphi_{c_1} + \varphi_{c_2}\right)\right] \tag{114}$$

$$\langle\langle J_{(a,\alpha),(2,2)} G^{A,(-1,-1,1,1)}_{[12],(\alpha,a),(2,2),(2),3} \rangle\rangle = J_0^{12} \langle\langle g^{A,2,2}_{\alpha,\beta} g^{A,2,1}_{b,b} g^{A,1,1}_{\beta,\gamma_{c_1}} g^{A,1,2}_{c_1,c_1} g^{A,2,2}_{\gamma_{c_1},\beta} g^{A,2,2}_{b,b} g^{A,2,2}_{\beta,\alpha} g^{A,2,1}_{a,a} g^{A,1,1}_{\alpha,\gamma_{c_2}} g^{A,1,2}_{c_2,c_2} g^{A,2,2}_{\gamma_{c_2},\alpha} g^{A,2,2}_{a,a} \rangle\rangle \tag{115}$$

$$= J_0^{12} \langle\langle g^{A,2,1}_{a,a} g^{A,2,2}_{a,a} \rangle\rangle \langle\langle g^{A,2,1}_{b,b} g^{A,2,2}_{b,b} \rangle\rangle \langle\langle g^{A,1,2}_{c_1,c_1} \rangle\rangle \langle\langle g^{A,1,2}_{c_2,c_2} \rangle\rangle \langle\langle g^{A,2,2}_{\alpha,\beta} g^{A,2,2}_{\beta,\alpha} \rangle\rangle \langle\langle g^{A,1,1}_{\alpha,\gamma_{c_2}} g^{A,2,2}_{\gamma_{c_2},\alpha} \rangle\rangle \langle\langle g^{A,1,1}_{\beta,\gamma_{c_1}} g^{A,2,2}_{\gamma_{c_1},\beta} \rangle\rangle \tag{116}$$

$$= -\frac{c_1}{32} \left(\frac{J_0}{W}\right)^{12} \frac{R_a R_b}{(l_e)^2} \frac{1}{k_F R_{\alpha,\beta}} \frac{1}{k_F R_{\alpha,\gamma_{c,2}}} \frac{1}{k_F R_{\beta,\gamma_{c,1}}} \frac{(\omega - i\eta)^2 \Delta^4}{\left(\Delta^2 - (\omega - i\eta)^2\right)^3} \exp\left[i\left(-\varphi_a - \varphi_b + \varphi_{c_1} + \varphi_{c_2}\right)\right] \tag{117}$$

$$\langle\langle J_{(a,\alpha),(2,2)} G^{A,(-1,-1,1,1)}_{[12],(\alpha,a),(2,2),(2),4} \rangle\rangle = J_0^{12} \langle\langle g^{A,2,2}_{\alpha,\beta} g^{A,2,1}_{b,b} g^{A,1,1}_{\beta,\gamma_{c_2}} g^{A,1,2}_{c_2,c_2} g^{A,2,2}_{\gamma_{c_2},\beta} g^{A,2,2}_{b,b} g^{A,2,2}_{\beta,\alpha} g^{A,2,1}_{a,a} g^{A,1,1}_{\alpha,\gamma_{c_1}} g^{A,1,2}_{c_1,c_1} g^{A,2,2}_{\gamma_{c_1},\alpha} g^{A,2,2}_{a,a} \rangle\rangle \tag{118}$$

$$= J_0^{12} \langle\langle g^{A,2,1}_{a,a} g^{A,2,2}_{a,a} \rangle\rangle \langle\langle g^{A,2,1}_{b,b} g^{A,2,2}_{b,b} \rangle\rangle \langle\langle g^{A,1,2}_{c_1,c_1} \rangle\rangle \langle\langle g^{A,1,2}_{c_2,c_2} \rangle\rangle \langle\langle g^{A,2,2}_{\alpha,\beta} g^{A,2,2}_{\beta,\alpha} \rangle\rangle \langle\langle g^{A,1,1}_{\alpha,\gamma_{c_1}} g^{A,2,2}_{\gamma_{c_1},\alpha} \rangle\rangle \langle\langle g^{A,1,1}_{\beta,\gamma_{c_2}} g^{A,2,2}_{\gamma_{c_2},\beta} \rangle\rangle \tag{119}$$

$$= -\frac{c_1}{32} \left(\frac{J_0}{W}\right)^{12} \frac{R_a R_b}{(l_e)^2} \frac{1}{k_F R_{\alpha,\beta}} \frac{1}{k_F R_{\alpha,\gamma_{c,1}}} \frac{1}{k_F R_{\beta,\gamma_{c,2}}} \frac{(\omega - i\eta)^2 \Delta^4}{\left(\Delta^2 - (\omega - i\eta)^2\right)^3} \exp\left[i\left(-\varphi_a - \varphi_b + \varphi_{c_1} + \varphi_{c_2}\right)\right] \tag{120}$$

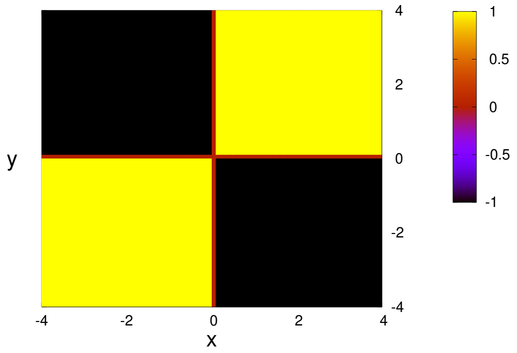


FIG. 2. In connection with Eq. (121), the colorplot shows $z(x,y) = \text{sign}\,[|x-y| - |x+y|]$ in the $(x,y)$ plane. It is seen that $z(x,y) = 1$ if $x$ and $y$ have the same sign, and $z(x,y) = -1$ otherwise.

## III. A USEFUL RELATION

A useful relation is established in this section, in connection with section VIII B in the paper.

The relation is the following: Take two real-valued variables $x$ and $y$, then:

$$|x+y| < |x-y| \iff x \text{ and } y \text{ have opposite signs.} \tag{121}$$

The demonstration is the following: If $x$ and $y$ are both positive, then $|x+y| = x+y$ and a contradiction is reached because $x+y$ cannot be smaller than $|x-y|$. A similar contradiction can be obtained for $x' = -x$ and $y' = -y$ in case $x$ and $y$ are both negative. The reverse can also be demonstrated easily: $x > 0$ and $y < 0$ with $x+y > 0$ implies necessarily $x+y < x-y$. On the other hand $x+y < 0$ and $x > 0$, $y < 0$ implies $-y > x$ and thus $-x-y < x-y$. The case $x < 0$ and $y > 0$ can be treated similarly upon exchanging $x$ and $y$ according to $x' = y$ and $y' = x$. Eq. (121) is confirmed by a numerical evaluation of $\text{sign}\,[|x-y| - |x+y|]$ in the $(x,y)$ plane (see figure 2).
